# Supplementary material for: The impact of locally-enhanced vertical diffusivity on the cross-shelf transport of tracers induced by a submarine canyon
Source: arXiv:1808.07237 ancillary file (2019-02-08)
Supplement: Supplementary file 1 [file sup_info.pdf]

# SUPPLEMENTAL INFORMATION TO "THE IMPACT OF LOCALLY-ENHANCED VERTICAL DIFFUSIVITY ON THE CROSS-SHELF TRANSPORT OF TRACERS INDUCED BY A SUBMARINE CANYON"

KARINA RAMOS-MUSALEM AND SUSAN E. ALLEN

Contents

1. Captions for animations 1
2. Additional figures 3
3. Complete tables 5
References 7

## 1. Captions for animations

**Animation S1.** This movie shows the concentration and near-bottom concentration for the canyon case as the upwelling event evolves. Top left and bottom right panels show alongshelf and cross-shelf sections of tracer concentration normalized by the initial values of concentration at each cell. This cross-sections are located at the dashed lines in the bottom left panel. The bottom left panel shows the bottom concentration normalized by the initial concentration at each cell close the shelf bottom. During the time dependent phase (spin-up of the shelf current) concentration near the canyon rim increases quickly. After day 4, concentration near the shelf, away from the canyon, slightly decreases because the canyon suppresses shelf-break upwelling, but the concentration near the rim and downstream keeps increasing.

**Animation S2.** This movie shows the relative increase in concentration and near-bottom concentration from the no-canyon case as the upwelling event evolves. Top left and bottom right panels show alongshelf and cross-shelf sections of tracer concentration anomaly (canyon minus no-canyon case) normalized by the initial values of concentration at each cell. This cross-sections are located at the dashed lines in the bottom left panel. The bottom left panel shows the bottom concentration anomaly normalized by the initial concentration at each cell close the shelf bottom. Compared to the no-canyon case, during the time dependent phase (spin-up of the shelf current) a large blob of water with higher-than-background concentrations upwells onto the shelf. This blob is sustained and fed by the upwelling flux through the canyon

and advected along the shelf during the advective phase (days 4-9); it can reach depths of 20 m above the bottom.

## 2. Additional figures

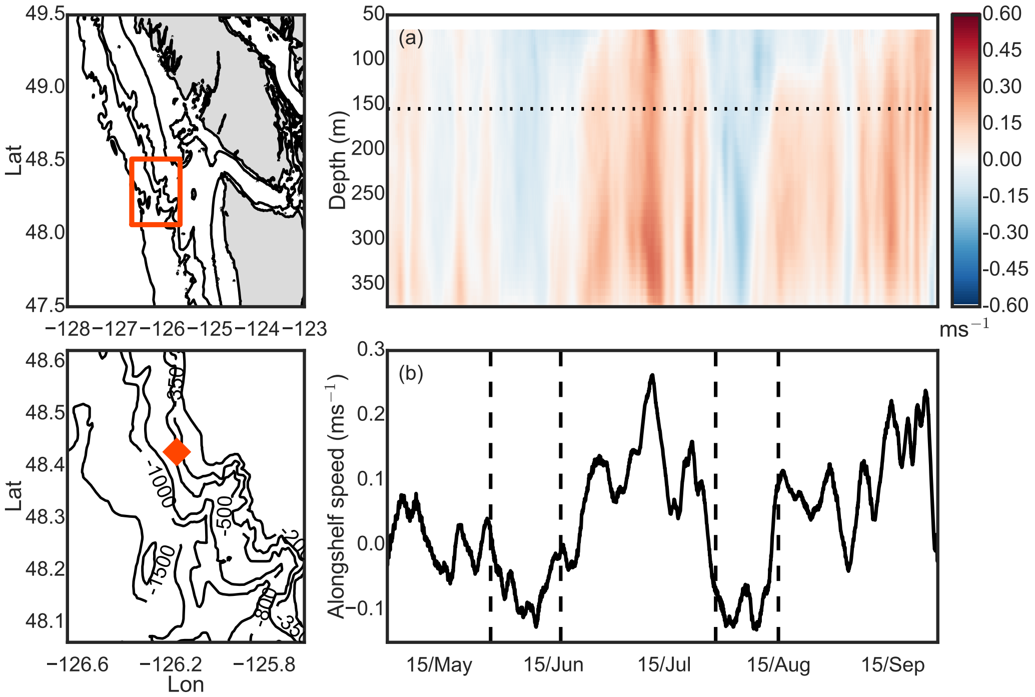


Figure S1. The main reason to choose simulations no longer than 9 days is that the time scale of upwelling events near the short canyons on the west coast of Vancouver Island, BC are on this order. To illustrate this, we show ADCP data at the slope on the west coast of Vancouver Island near Barkley Canyon. Alongshelf and cross-shore velocities were provided by the Neptune Observatory operated by Ocean Networks Canada at Pod 2 of the upper slope station of the Barkley Canyon network, taken from the 75kHz ADCP located at 400 m depth, upstream of Barkley Canyon, during upwelling conditions. The alongshore velocity was filtered using a Doodson filter (39 hours) to remove the tides. Although summer 2014 was not particularly upwelling favourable, we see two longer events, one from May 29th to June 17th and the second one from July 29th to August 15th (b). Each one lasts no more than 20 days each. This is consistent with evidence reported by Mirshak and Allen (2005) and Hickey (1997). Also note that the flow is nearly-uniform in the vertical between 50-250 m depth during the two periods of canyon-driven upwelling favourable flow, supporting the use of body forcing to generate a deeper shelf current than wind stress would (a). Negative (upwelling-favourable) flows are directed southwards.

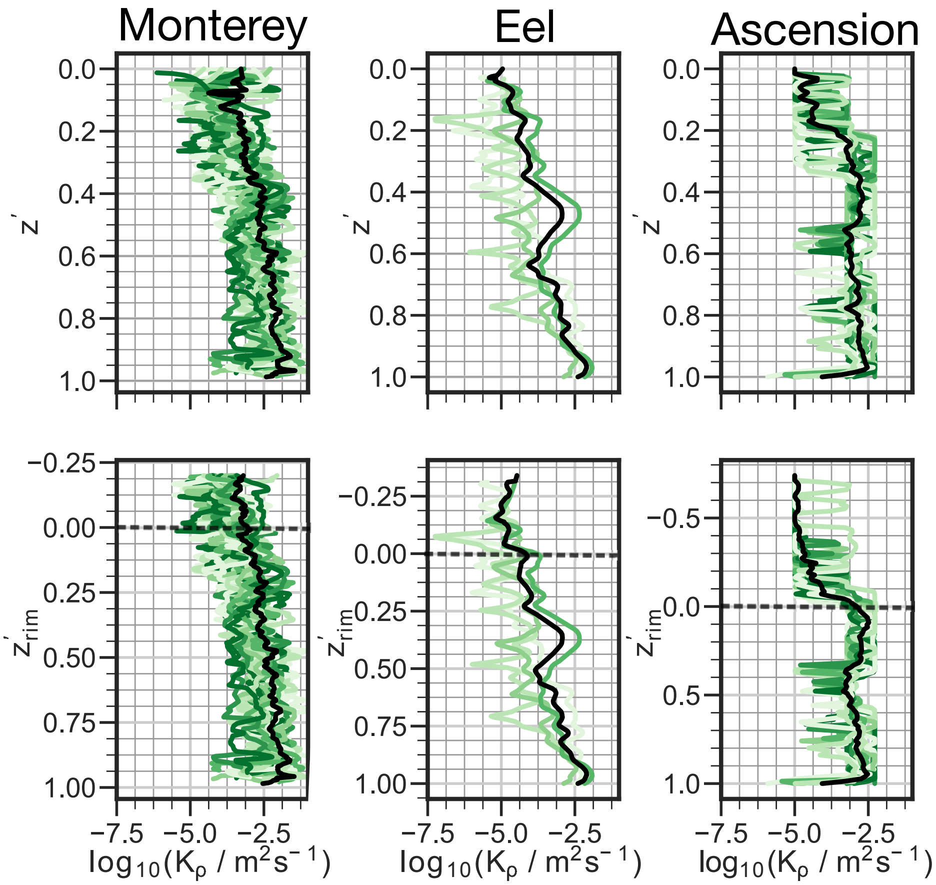


FIGURE S2. Diffusivity profiles from observations in Monterey (Carter and Gregg, 2002) , Eel (Waterhouse et al., 2017) and Ascension (Gregg et al., 2011) Canyons. Green lines correspond to individual profiles along the canyon axis and black lines correspond to the mean profile. For comparison, the vertical coordinate is normalized in two different ways: by bottom depth, $z' = z/z_{bottom}$ where $z_{bottom}$ is the depth of the canyon at each particular station; or using the rim depth, $z'_{rim} = (z - z_{rim})/(z_{bottom} - z_{rim})$. We run simulations with both normalizations for each canyon. Note that for Monterey and Ascension Canyons, the mean profiles have similar levels of diffusivity near rim depth ($z'_{rim} = 0$, dashed black line) to our locally-enhanced diffusivity runs. We assigned values of $\epsilon$ to each run based on the variation of $K_v$ above rim depth and found it to be on the order of 50 m. Data from Monterey and Eel Canyons were kindly provided by G. Carter and A. Waterhouse, respectively. Profiles from Ascension Canyon were taken directly from Figure 11 in (Gregg et al., 2011) by using an inverse algorithm on the image, so the accuracy of the data is not what is reported on the original paper. We are using these data to put our experiments into context and compare it to less idealized mixing profiles.

## 3. Complete tables

Table S1. Mean vertical (VTT), advective (VATT) and total (TTT) tracer transport anomalies through cross sections CS1-CS5 and LID as well as vertical water (VWT) and total (TWT) water transport anomalies throughout the advective phase with corresponding standard deviations calculated as 12 hour variations for all runs.

| Exp | VTT $10^5\ \mu$Mm$^3$s$^{-1}$ | VATT $10^5\ \mu$Mm$^3$s$^{-1}$ | TTT $10^4\ \mu$Mm$^3$s$^{-1}$ | VWT $10^4$ m$^3$s$^{-1}$ | TWT $10^2$ m$^3$s$^{-1}$ |
|---|---|---|---|---|---|
| base case | 1.6±0.29 | 1.6±0.29 | 0.46±0.13 | 1.9±0.46 | -1.6±5.2 |
| $\uparrow N_0$ | 1.1±0.24 | 1.1±0.24 | 0.29±0.09 | 1.4±0.36 | -2.4±6.0 |
| $\uparrow\uparrow N_0$ | 0.73±0.20 | 0.73±0.20 | 0.14±0.06 | 0.91±0.29 | -5.5±4.7 |
| $\Downarrow N_0$ | 2.3±0.40 | 2.3±0.40 | 0.79±0.18 | 2.5±0.61 | -1.4±3.3 |
| $\downarrow\downarrow N_0$ | 2.2±0.36 | 2.2±0.36 | 0.74±0.16 | 2.5±0.58 | -1.4±4.0 |
| $\uparrow f$ | 1.7±0.32 | 1.7±0.32 | 0.49±0.13 | 2.0±0.48 | -0.57±5.04 |
| $\downarrow\downarrow f$ | 1.1±0.17 | 1.1±0.17 | 0.30±0.10 | 1.3±0.33 | -11.4±6.2 |
| $\downarrow f$ | 1.3±0.22 | 1.3±0.22 | 0.37±0.11 | 1.6±0.39 | -6.1±5.7 |
| $\Downarrow f$ | 0.92±0.16 | 0.92±0.16 | 0.21±0.09 | 1.0±0.32 | -18.1±6.5 |
| $\downarrow$ U | 1.4±0.29 | 1.4±0.29 | 0.38±0.09 | 1.7±0.48 | 0.61±6.8 |
| $\downarrow\downarrow$ U | 1.1±0.26 | 1.1±0.26 | 0.27±0.06 | 1.4±0.39 | -0.55±5.8 |
| $\Downarrow$ U | 0.43±0.05 | 0.43±0.05 | 0.12±0.01 | 0.60±0.09 | 4.3±2.2 |
| $\Downarrow$ U, $\downarrow\downarrow N_0$ | 0.72±0.04 | 0.72±0.04 | 0.21±0.01 | 0.94±0.08 | 5.9±2.1 |
| $\Downarrow$ U, $\uparrow\uparrow N_0$ | 0.21±0.04 | 0.21±0.04 | 0.06±0.01 | 0.32±0.06 | 3.4±1.2 |
| $\Downarrow$ U, $\Downarrow f$ | 0.26±0.04 | 0.26±0.04 | 0.06±0.01 | 0.37±0.07 | 0.91±2.2 |
| $\Uparrow\Uparrow K_{can}$, $\epsilon$10 | 2.2±0.21 | 1.9±0.21 | 1.1±0.09 | 2.2±0.28 | 8.5±1.3 |
| $\Uparrow\Uparrow K_{can}$, $\epsilon$25 | 2.5±0.18 | 2.2±0.18 | 1.2±0.06 | 2.4±0.24 | 4.6±1.1 |
| $\Uparrow\Uparrow K_{can}$, $\epsilon$50 | 2.8±0.15 | 2.5±0.16 | 1.3±0.06 | 2.8±0.22 | 3.0±1.3 |
| $\Uparrow\Uparrow K_{can}$, $\epsilon$100 | 3.0±0.15 | 2.6±0.16 | 1.3±0.08 | 3.0±0.21 | 1.8±1.3 |
| $\Uparrow\Uparrow K_{can}$, $\epsilon$15 | 2.4±0.20 | 2.0±0.20 | 1.2±0.08 | 2.3±0.27 | 7.5±1.05 |
| $\Uparrow\Uparrow K_{can}$, $\epsilon$75 | 2.9±0.14 | 2.5±0.16 | 1.3±0.07 | 2.9±0.21 | 2.2±1.3 |
| $\uparrow\uparrow K_{can}$ | 1.9±0.25 | 1.8±0.25 | 0.74±0.10 | 2.1±0.39 | 0.64±3.7 |
| $\Uparrow\uparrow K_{can}$ | 2.2±0.22 | 2.0±0.22 | 1.0±0.09 | 2.4±0.32 | 7.7±2.5 |
| $\uparrow\uparrow K_{can}$ $\epsilon$25 | 1.9±0.25 | 1.8±0.26 | 0.71±0.10 | 2.1±0.40 | -0.70±4.2 |
| $\uparrow\uparrow K_{can}$ $\epsilon$100 | 1.9±0.25 | 1.8±0.25 | 0.69±0.10 | 2.1±0.40 | -1.6±3.8 |
| $\Uparrow\uparrow K_{can}$ $\epsilon$25 | 2.4±0.20 | 2.1±0.20 | 1.1±0.07 | 2.4±0.31 | 2.14±2.01 |
| $\Uparrow\uparrow K_{can}$, $\epsilon$100 | 2.5±0.18 | 2.3±0.19 | 1.1±0.07 | 2.7±0.29 | 0.36±1.9 |
| $\Uparrow\uparrow\uparrow K_{can}$ | 2.2±0.25 | 1.9±0.24 | 1.0±0.10 | 2.2±0.32 | 9.5±2.2 |
| $\Uparrow\Uparrow\uparrow K_{can}$ | 1.9±0.25 | 1.7±0.23 | 0.94±0.11 | 1.9±0.30 | 9.7±1.5 |
| $\Uparrow K_{can}$ | 2.1±0.22 | 2.0±0.23 | 0.91±0.08 | 2.3±0.34 | 4.2±2.9 |
| $\uparrow K_{can}$ | 1.8±0.26 | 1.7±0.26 | 0.65±0.11 | 2.0±0.42 | -0.55±4.4 |
| $\Uparrow\Uparrow K_{can}$ | 2.0±0.25 | 1.8±0.24 | 0.97±0.11 | 2.1±0.32 | 9.6±1.8 |

TABLE S2. Mean water and tracer upwelling fluxes ($\Phi$ (4) and $\Phi_{Tr}$ (5)) for selected runs during the advective phase, reported with 12 hour standard deviations. All other quantities are evaluated at day 9: Volume of upwelled water ($V_{can}$), upwelled tracer ($M_{can}$) for the canyon case and fractional canyon contributions to these quantities calculated as the canyon case minus the no-canyon case divided by the canyon case, and total tracer mass anomaly on shelf ($\mathcal{M}$-$\mathcal{M}_{nc}$ (6)) in kg of $NO^{-}{}_3$.

| Exp | $\Phi$ ($10^4$ m$^3$s$^{-1}$) | $\Phi_{Tr}$ ($10^5$ $\mu$Mm$^3$s$^{-1}$) | $V_{can}$ ($10^{10}$ m$^3$) | ($V_{can}$ − $V_{nc}$) $V_{can}^{-1}$ (%) | $M_{can}$ ($10^{11}$ $\mu$Mm$^3$) | ($M_{can}$ − $M_{nc}$) $M_{can}^{-1}$ (%) | $\mathcal{M} - \mathcal{M}_{nc}$ ($10^6$ kg $NO_3^-$) |
|---|---|---|---|---|---|---|---|
| base case | 3.85±0.60 | 2.76± 0.26 | 2.86 | 81.61 | 2.20 | 82.57 | 1.96 |
| $\uparrow K_{bg}$ | 3.70±0.73 | 2.29± 0.24 | 2.80 | 87.26 | 2.05 | 87.20 | 2.02 |
| $\uparrow\uparrow K_{bg}$ | 3.72±1.58 | 0.96± 0.40 | 3.12 | 63.77 | 1.79 | 58.68 | 2.35 |
| $\uparrow N_0$ | 2.86±0.44 | 1.99± 0.19 | 2.08 | 88.29 | 1.57 | 88.52 | 1.21 |
| $\uparrow\uparrow N_0$ | 1.32±0.55 | 1.11± 0.44 | 1.10 | 77.74 | 0.82 | 77.91 | 0.62 |
| $\Downarrow N_0$ | 6.78±0.94 | 5.21± 0.82 | 4.63 | 29.03 | 3.69 | 34.85 | 3.48 |
| $\downarrow\downarrow N_0$ | 6.34±0.92 | 4.84± 0.72 | 4.35 | 30.84 | 3.45 | 36.36 | 3.25 |
| $\downarrow N_0$ | 5.15±0.95 | 3.86± 0.74 | 3.69 | 35.50 | 2.90 | 40.33 | 2.73 |
| $\uparrow f$ | 4.03±0.58 | 2.95± 0.36 | 2.96 | 73.08 | 2.30 | 74.70 | 2.06 |
| $\downarrow\downarrow f$ | 2.95±0.72 | 1.96± 0.33 | 2.18 | 85.80 | 1.65 | 86.09 | 1.38 |
| $\downarrow f$ | 3.42±0.73 | 2.28± 0.14 | 2.51 | 88.28 | 1.92 | 88.62 | 1.64 |
| $\Downarrow f$ | 1.83±0.88 | 1.03± 0.42 | 1.56 | 76.77 | 1.17 | 77.09 | 1.03 |
| $\downarrow$ U | 3.02±0.39 | 2.27± 0.27 | 2.18 | 86.87 | 1.66 | 87.30 | 1.48 |
| $\downarrow\downarrow$ U | 1.92±0.39 | 1.50± 0.26 | 1.41 | 82.16 | 1.06 | 82.63 | 1.03 |
| $\Downarrow$ U | 0.14±0.23 | 0.15± 0.07 | 0.18 | 69.05 | 0.13 | 69.53 | 0.31 |
| $\Downarrow$ U, $\downarrow\downarrow N_0$ | 0.61±0.27 | 0.40± 0.12 | 0.49 | 66.83 | 0.37 | 67.73 | 0.59 |
| $\Downarrow$ U, $\uparrow\uparrow N_0$ | 0.01±0.07 | -0.02± 0.02 | 0.03 | 40.56 | 0.02 | 41.18 | 0.13 |
| $\Downarrow$ U, $\Downarrow f$ | 0.11±0.35 | -0.02± 0.04 | 0.10 | 17.99 | 0.08 | 18.79 | 0.18 |
| $\Downarrow$ U, $\uparrow\uparrow K_{can}$ | 1.23±0.46 | 0.74± 0.09 | 0.88 | 0.78 | 0.65 | 1.26 | 0.25 |
| $K_{can}$ Monterey (bot) | 4.97±0.48 | 3.77± 0.31 | 3.62 | 85.48 | 2.71 | 85.81 | 4.57 |
| $K_{can}$ Eel (bot) | 3.86±0.59 | 2.74± 0.20 | 2.89 | 81.81 | 2.22 | 82.69 | 2.81 |
| $K_{can}$ Monterey | 3.87±0.53 | 2.80± 0.16 | 2.87 | 81.69 | 2.25 | 82.94 | 2.85 |
| $K_{can}$ Ascension (bot) | 4.18±0.60 | 3.01± 0.24 | 3.07 | 82.91 | 2.37 | 83.82 | 3.29 |
| $\Uparrow\Uparrow K_{can}$, $\epsilon$10 | 4.07±0.55 | 3.42± 0.34 | 3.10 | 83.05 | 2.53 | 84.83 | 3.71 |
| $\Uparrow\Uparrow K_{can}$, $\epsilon$25 | 4.12±0.71 | 3.43± 0.50 | 3.14 | 83.29 | 2.52 | 84.76 | 4.24 |
| $\Uparrow\Uparrow K_{can}$, $\epsilon$50 | 4.21±0.71 | 3.29± 0.55 | 3.18 | 83.48 | 2.46 | 84.38 | 4.53 |
| $\Uparrow\Uparrow K_{can}$, $\epsilon$100 | 4.51±0.64 | 3.40± 0.46 | 3.36 | 84.37 | 2.52 | 84.76 | 4.70 |
| $\Uparrow\Uparrow K_{can}$, $\epsilon$15 | 4.08±0.65 | 3.47± 0.41 | 3.12 | 83.17 | 2.54 | 84.89 | 3.94 |
| $\Uparrow\Uparrow K_{can}$, $\epsilon$75 | 4.39±0.67 | 3.36± 0.50 | 3.28 | 84.01 | 2.49 | 84.57 | 4.63 |
| $\Uparrow\Uparrow K_{can}$, $\epsilon$150 | 4.70±0.61 | 3.50± 0.40 | 3.45 | 84.80 | 2.56 | 85.00 | 4.71 |
| $\uparrow\uparrow K_{can}$ | 3.77±0.62 | 2.71± 0.13 | 2.84 | 81.53 | 2.24 | 82.83 | 2.77 |
| $\Uparrow\uparrow K_{can}$ | 4.05±0.50 | 3.21± 0.29 | 3.03 | 82.65 | 2.46 | 84.35 | 3.50 |
| $\uparrow\uparrow K_{can}$ $\epsilon$25 | 3.73±0.63 | 2.65± 0.13 | 2.82 | 81.41 | 2.21 | 82.60 | 2.70 |
| $\uparrow\uparrow K_{can}$ $\epsilon$100 | 3.70±0.67 | 2.57± 0.17 | 2.81 | 81.34 | 2.17 | 82.31 | 2.66 |
| $\Uparrow\uparrow K_{can}$ $\epsilon$25 | 3.98±0.53 | 3.09± 0.30 | 3.00 | 82.47 | 2.39 | 83.91 | 3.73 |
| $\Uparrow\uparrow K_{can}$, $\epsilon$100 | 4.14±0.56 | 3.04± 0.27 | 3.07 | 82.92 | 2.35 | 83.63 | 3.86 |
| $\Uparrow\uparrow\uparrow K_{can}$ | 4.08±0.54 | 3.35± 0.33 | 3.08 | 82.94 | 2.51 | 84.70 | 3.48 |
| $\Uparrow\Uparrow\uparrow K_{can}$ | 4.17±0.65 | 3.51± 0.39 | 3.13 | 83.22 | 2.55 | 84.95 | 3.27 |
| $\Uparrow K_{can}$ | 3.91±0.56 | 2.93± 0.16 | 2.92 | 82.03 | 2.34 | 83.57 | 3.23 |
| $\uparrow K_{can}$ | 3.65±0.67 | 2.57± 0.13 | 2.78 | 81.14 | 2.17 | 82.33 | 2.50 |
| $\Uparrow\Uparrow K_{can}$ | 4.09±0.58 | 3.39± 0.37 | 3.09 | 83.02 | 2.53 | 84.79 | 3.38 |

## References

Carter, G. S. and Gregg, M. C. (2002). Intense, Variable Mixing near the Head of Monterey Submarine Canyon. *J. Phys. Oceanogr.*, 32:3145–3165.

Gregg, M. C., Hall, R. a., Carter, G. S., Alford, M. H., Lien, R.-C., Winkel, D. P., and Wain, D. J. (2011). Flow and mixing in Ascension, a steep, narrow canyon. *J. Geophys. Res.*, 116:C07016.

Hickey, B. M. (1997). The Response of a Steep-Sided, Narrow Canyon to Time-Variable Wind Forcing. *J. Phys. Oceanogr.*, 27:697–726.

Mirshak, R. and Allen, S. E. (2005). Spin-up and the effects of a submarine canyon: Applications to upwelling in Astoria Canyon. *J. Geophys. Res.*, 110:C02013.

Waterhouse, A. F., Mackinnon, J. A., Musgrave, R. C., Kelly, S. M., Pickering, A., and Nash, J. (2017). Internal Tide Convergence and Mixing in a Submarine Canyon. *J. Phys. Oceanogr.*, 47:303–322.
